# Supplementary material for: ThinkBot: Embodied Instruction Following with Thought Chain Reasoning
Source: arXiv:2312.07062 source file (2023-12-14)
Supplement: Supplementary file 1 [file X_suppl.tex]

\clearpage
\setcounter{page}{1}
\maketitlesupplementary

In this supplementary material, we provide additional details and experiments not included in the main paper due to limitations in space.
\begin{itemize}
    % \item \Cref{a:related_work}: More related work.
    % multi-modal localizer v.s. sem policy of FILM
    \item \Cref{a:alfred}: Details of the ALFRED benchmark and the hard valid unseen split used in our experiments.
    \item \Cref{a:prompter_plus}: Details of the Prompter+ baseline, a modified version we implement based on Prompter \cite{inoue2022prompter}.
    \item \Cref{a:full_prompt}: The entire system message template for the instruction completer in our \method.
    \item \Cref{a:additional_quantitative}: Supplementary quantitative analysis.
    \item \Cref{a:additional_qualitative}: Supplementary qualitative analysis.
\end{itemize}

\section{Details of the ALFRED Benchmark}   % CPEM
\label{a:alfred}

In this section, we first provide a concise overview of the input and output space within the ALFRED benchmark, and then analyze the hard valid unseen split we extracted from the valid unseen split.

In a typical ALFRED task, the agent is spawned into a 3D indoor floor plan with a first-person view.
% input space
To specify a task, the agent receives a high-level goal statement that describes the task's objective and step-by-step instruction that provides detailed explanations.
Accompanying these, the agent receives a $300\times300$ egocentric RGB frame and outputs actions for each time step.
Note that during the test phase, other information such as groundtruth depth images and instance segmentation images is not provided to the agent.
% output space
The action space of the agent consists of \num{5} navigation actions, \num{7} interaction actions, and a \textsc{Stop} action.
The navigation actions are \textsc{MoveAhead}, \textsc{RotateLeft}, \textsc{RotateRight}, \textsc{LookUp}, and \textsc{LookDown}. 
The interaction actions are \textsc{PickupObject}, \textsc{PutObject}, \textsc{OpenObject}, \textsc{CloseObject}, \textsc{ToggleObjectOn}, \textsc{ToggleObjectOff}, and \textsc{SliceObject}.
If an interaction action is outputted, the agent is required to predict an additional binary object mask for the current RGB frame, so that the agent can interact with the object of the highest IoU score.
When the agent takes the \textsc{Stop} action, the simulator will check whether all objects are correctly positioned based on a predefined PDDL domain. The trial will fail if the agent exceeds the \num{1000}-step limit or makes more than \num{10} errors while attempting to achieve the goal.

As outlined in the main paper, we have created a specific subset named \emph{hard valid unseen} split from the valid unseen split in ALFRED.
The hard valid unseen split only includes cases where all target objects are confined within closed containers, to assess the agent's capability to recover missing interactions.
These types of cases make up 8.6\% in the valid unseen split, 4.8\% in the valid seen split, and 5.52\% in the train split, indicating the importance for the agent to handle such situations.
Consequently, the hard valid unseen split contains \num{74} trials extracted from the valid unseen split, involving five task types of `Examine', `Pick \& Place', `Stack \& Place', `Clean \& Place' and `Heat \& Place'. The hard valid unseen split is capable of evaluating the agent's ability to recover missing interactions comprehensively.

\begin{table}[t!]
    \footnotesize
    \centering
    \setlength\tabcolsep{3pt}
    \begin{tabular}{lcccc}
    \toprule
    \textbf{Error mode} & FILM & Prompter & Prompter+ & \textbf{\method} (Ours) \\
    \midrule
    Goal object not found & 53.01 & 34.39 & 21.10 & 18.08 \\
    Interaction failures & 6.78 & 7.72 & 7.56 & 7.32 \\
    Navigation failures & 19.60 & 4.62 & 6.95 & 6.83 \\
    \bottomrule
    \end{tabular}
    % \caption{\textbf{Comparisons of error modes}. Note that we fold the `Object in a closed confinement' and `Language processing' error from their paper \cite{min2022film, inoue2022prompter} into `Goal object not found' and `Others' here, respectively.}
    \caption{Comparisons of error modes. Note that we fold the `Object in a closed confinement' and `Language processing' errors from \cite{min2022film, inoue2022prompter} into `Goal object not found' error, and fold `Collisions' and `Others' errors into `Navigation failures' error here.}
    %our \method performs better in dealing with `Goal Object not found' error, which is the dominant error of the counterparts.}
    \label{a:table:error_modes}
    \vspace{-0.1cm}
\end{table}

\section{Details of the Prompter+ Baseline}
\label{a:prompter_plus}
% \footnote{\url{https://github.com/hitachi-rd-cv/prompter-alfred}}
% We do not do any hyper-parameter search, so the performance of the detector can be further improved.
In the main paper, we have constructed a strong baseline termed Prompter+, and we provide additional implementation details of Prompter+ in this section.
Prompter+ is built upon the Prompter codebase, which combines environment-aware memory \cite{kim2023context} and a re-trained object detector \cite{wang2023internimage} with the vanilla Prompter.
We utilize the InternImage-XL backbone pretrained on the COCO dataset \cite{lin2014microsoft} with Cascade Mask R-CNN head implemented \cite{wang2023internimage} on MMDetection \cite{mmdetection}.
To collect the dataset for finetuning, we replay the expert trajectories in the ALFRED train split, and record the egocentric image and the groundtruth instance mask at each step.
Following \cite{ALFWorld20}, we also balance the training samples from each room type in the ALFRED benchmark.
For finetuning, we use AdamW optimizer \cite{loshchilov2017decoupled} with an initial learning rate of \num{1e-4} and weight decay of \num{5e-2}. Please refer to \cite{wang2023internimage} for more training details.
The whole finetuning process takes one day on 4 NVIDIA 3090 GPUs, where the batch size on each GPU is set to 4.

% We compare the instance segmentation performance of the Mask R-CNN with ResNet50 backbone in \cite{ALFWorld20, min2022film, inoue2022prompter} and InternImage model finetuned on the same validation dataset we collect from the ALFRED valid unseen split.
% Note that we train separate models for small objects and large receptacles following \cite{ALFWorld20, min2022film}.
% As shown in \Cref{a:table:seg}, the InternImage-XL model significantly surpasses the Mask R-CNN used in \cite{ALFWorld20, min2022film}. 
% For example, the box AP (\ie $\rm AP^b$ in \Cref{a:table:seg}) of InternImage-XL is 19.8 better than Mask R-CNN (93.7 vs. 73.9).
% The results demonstrate the superiority of the instance segmentation model we re-train for the Prompter+.

\section{Full Prompt of the Instruction Completer}
\label{a:full_prompt}

\begin{table*}[t!]
\footnotesize
\centering
\setlength\tabcolsep{9pt}
\begin{tabular}{lccccccc}
\toprule
\textbf{Method} & Examine & Pick \& Place & Stack \& Place & Clean \& Place & Cool \& Place & Heat \& Place & Pick 2 \& Place \\
\midrule
Seq2seq & 0 & 0 & 0 & 0 & 0 & 0 & 0 \\
MOCA & 4.6 & 6.0 & 6.4 & 10.6 & 2.8 & 5.1 & 1.2 \\
\midrule
HLSM & 36.6 & 34.8 & 4.4 & 11.3 & 14.8 & 0.0 & 18.0 \\
FILM & 29.7 & 16.0 & 2.0 & 33.6 & 14.0 & 23.0 & 11.8 \\
Prompter+ & \textbf{80.9} & 46.0 & 32.1 & 71.7 & 82.6 & 78.7 & \textbf{37.0} \\
\midrule
% \rowcolor{gray!10}
\textbf{\method} (Ours) & 79.2 & \textbf{50.0} & \textbf{40.4} & \textbf{77.9} & \textbf{88.1} & \textbf{86.0} & 33.3 \\
\bottomrule
\end{tabular}
\caption{Comparisons with the state-of-the-art methods in success rate on the valid unseen split break down by task type.}    
\label{a:table:task_type}
\end{table*}

\begin{figure*}[t!]
    \small
    \centering
    \includegraphics[width=\linewidth]{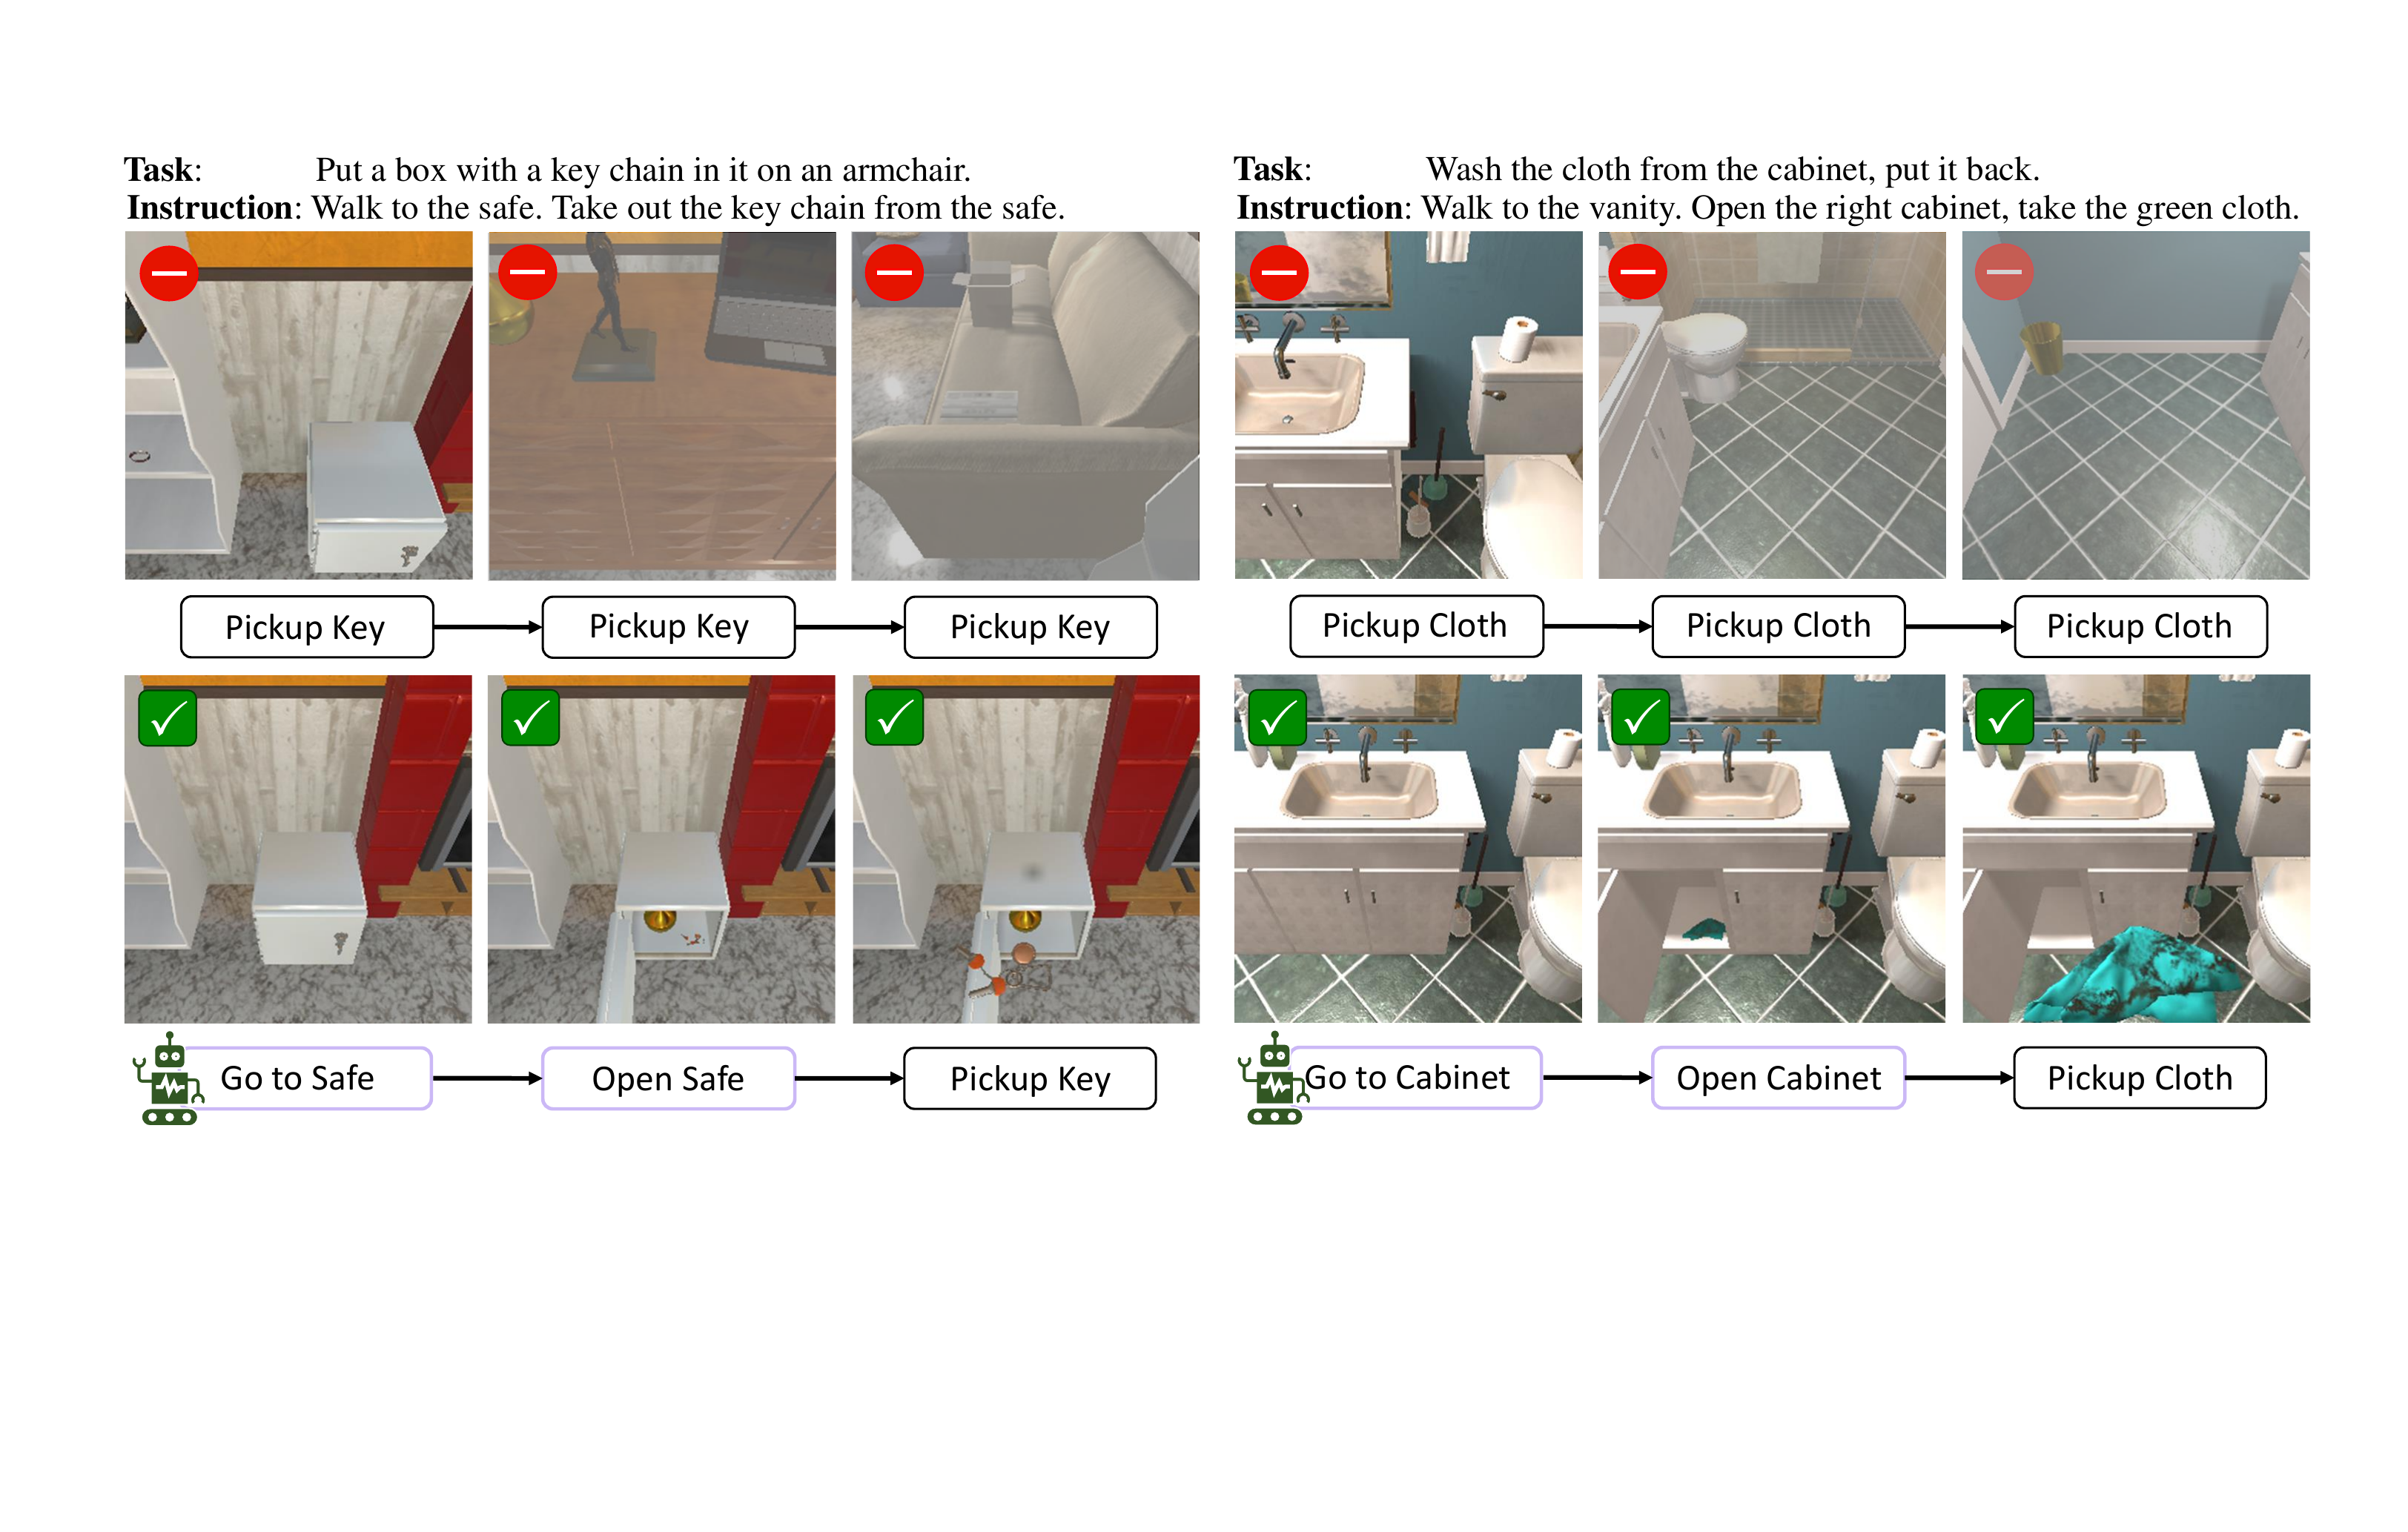}
    \vspace{-0.1cm}
    \caption{Visualization of the agent action sequences acquired by Prompter+ (top) and our ThinkBot (bottom), where our method can recover the missing actions with interacted instances `Open Safe' and `Open Cabinet' to successfully achieve the human goal.}
    % \vspace{-1em}
    % \vspace{-0.1cm}
    \label{a:fig:qualitative_a_sequence}
\end{figure*}

In this section, we present the full system prompt for the instruction completer in our \method for reproducibility. 

\subsection{Components in the Prompt}
The system prompt template for our instruction completer consists of the following components: 
\begin{enumerate}[label=(\arabic*)]
    \item The role explanation with the emotion prompt \cite{li2023emotionprompt}; 
    \item Definition of the task description:\begin{itemize}
        \item High-level goal statement: A string describes the goal of this household task.
        \item Low-level step-by-step instruction: A list contains the whole incoherent human instruction.
        \item Possible landmarks in this room type: A list contains all possible landmarks in the current room to avoid object hallucination.
        \item Task Completion: The current task completion progress we provide for the agent to locate the corresponding instruction sentences.
    \end{itemize}
    \item Definition of the agent's current state:\begin{itemize}
        \item Global observed landmarks: A list of observed landmarks, \eg, [`CounterTop', `StoveBurner'];
        \item Last message: A string contains the failure message from the last run.
    \end{itemize}
    \item Primitive actions: All interaction actions and the related arguments we introduce in \Cref{a:alfred} along with a `GotoLocation' subgoal for navigation.
    \vspace{0.07cm}
    \item Requirements on the response format, where we impose chain-of-thought prompting~\cite{wei2022chain}: We request the large language model to first reason on the current subtask then give a detailed action list. The last predicted subgoal should always be the same as the current subgoal for coherent instruction recovery.
\end{enumerate}

\subsection{Full Prompt}
The complete system prompt template is shown in \Cref{a:system_prompt}, and the response format is shown in \Cref{a:response_format}.

\begin{figure*}[t!]
    \small
    \centering
    \includegraphics[width=\linewidth]{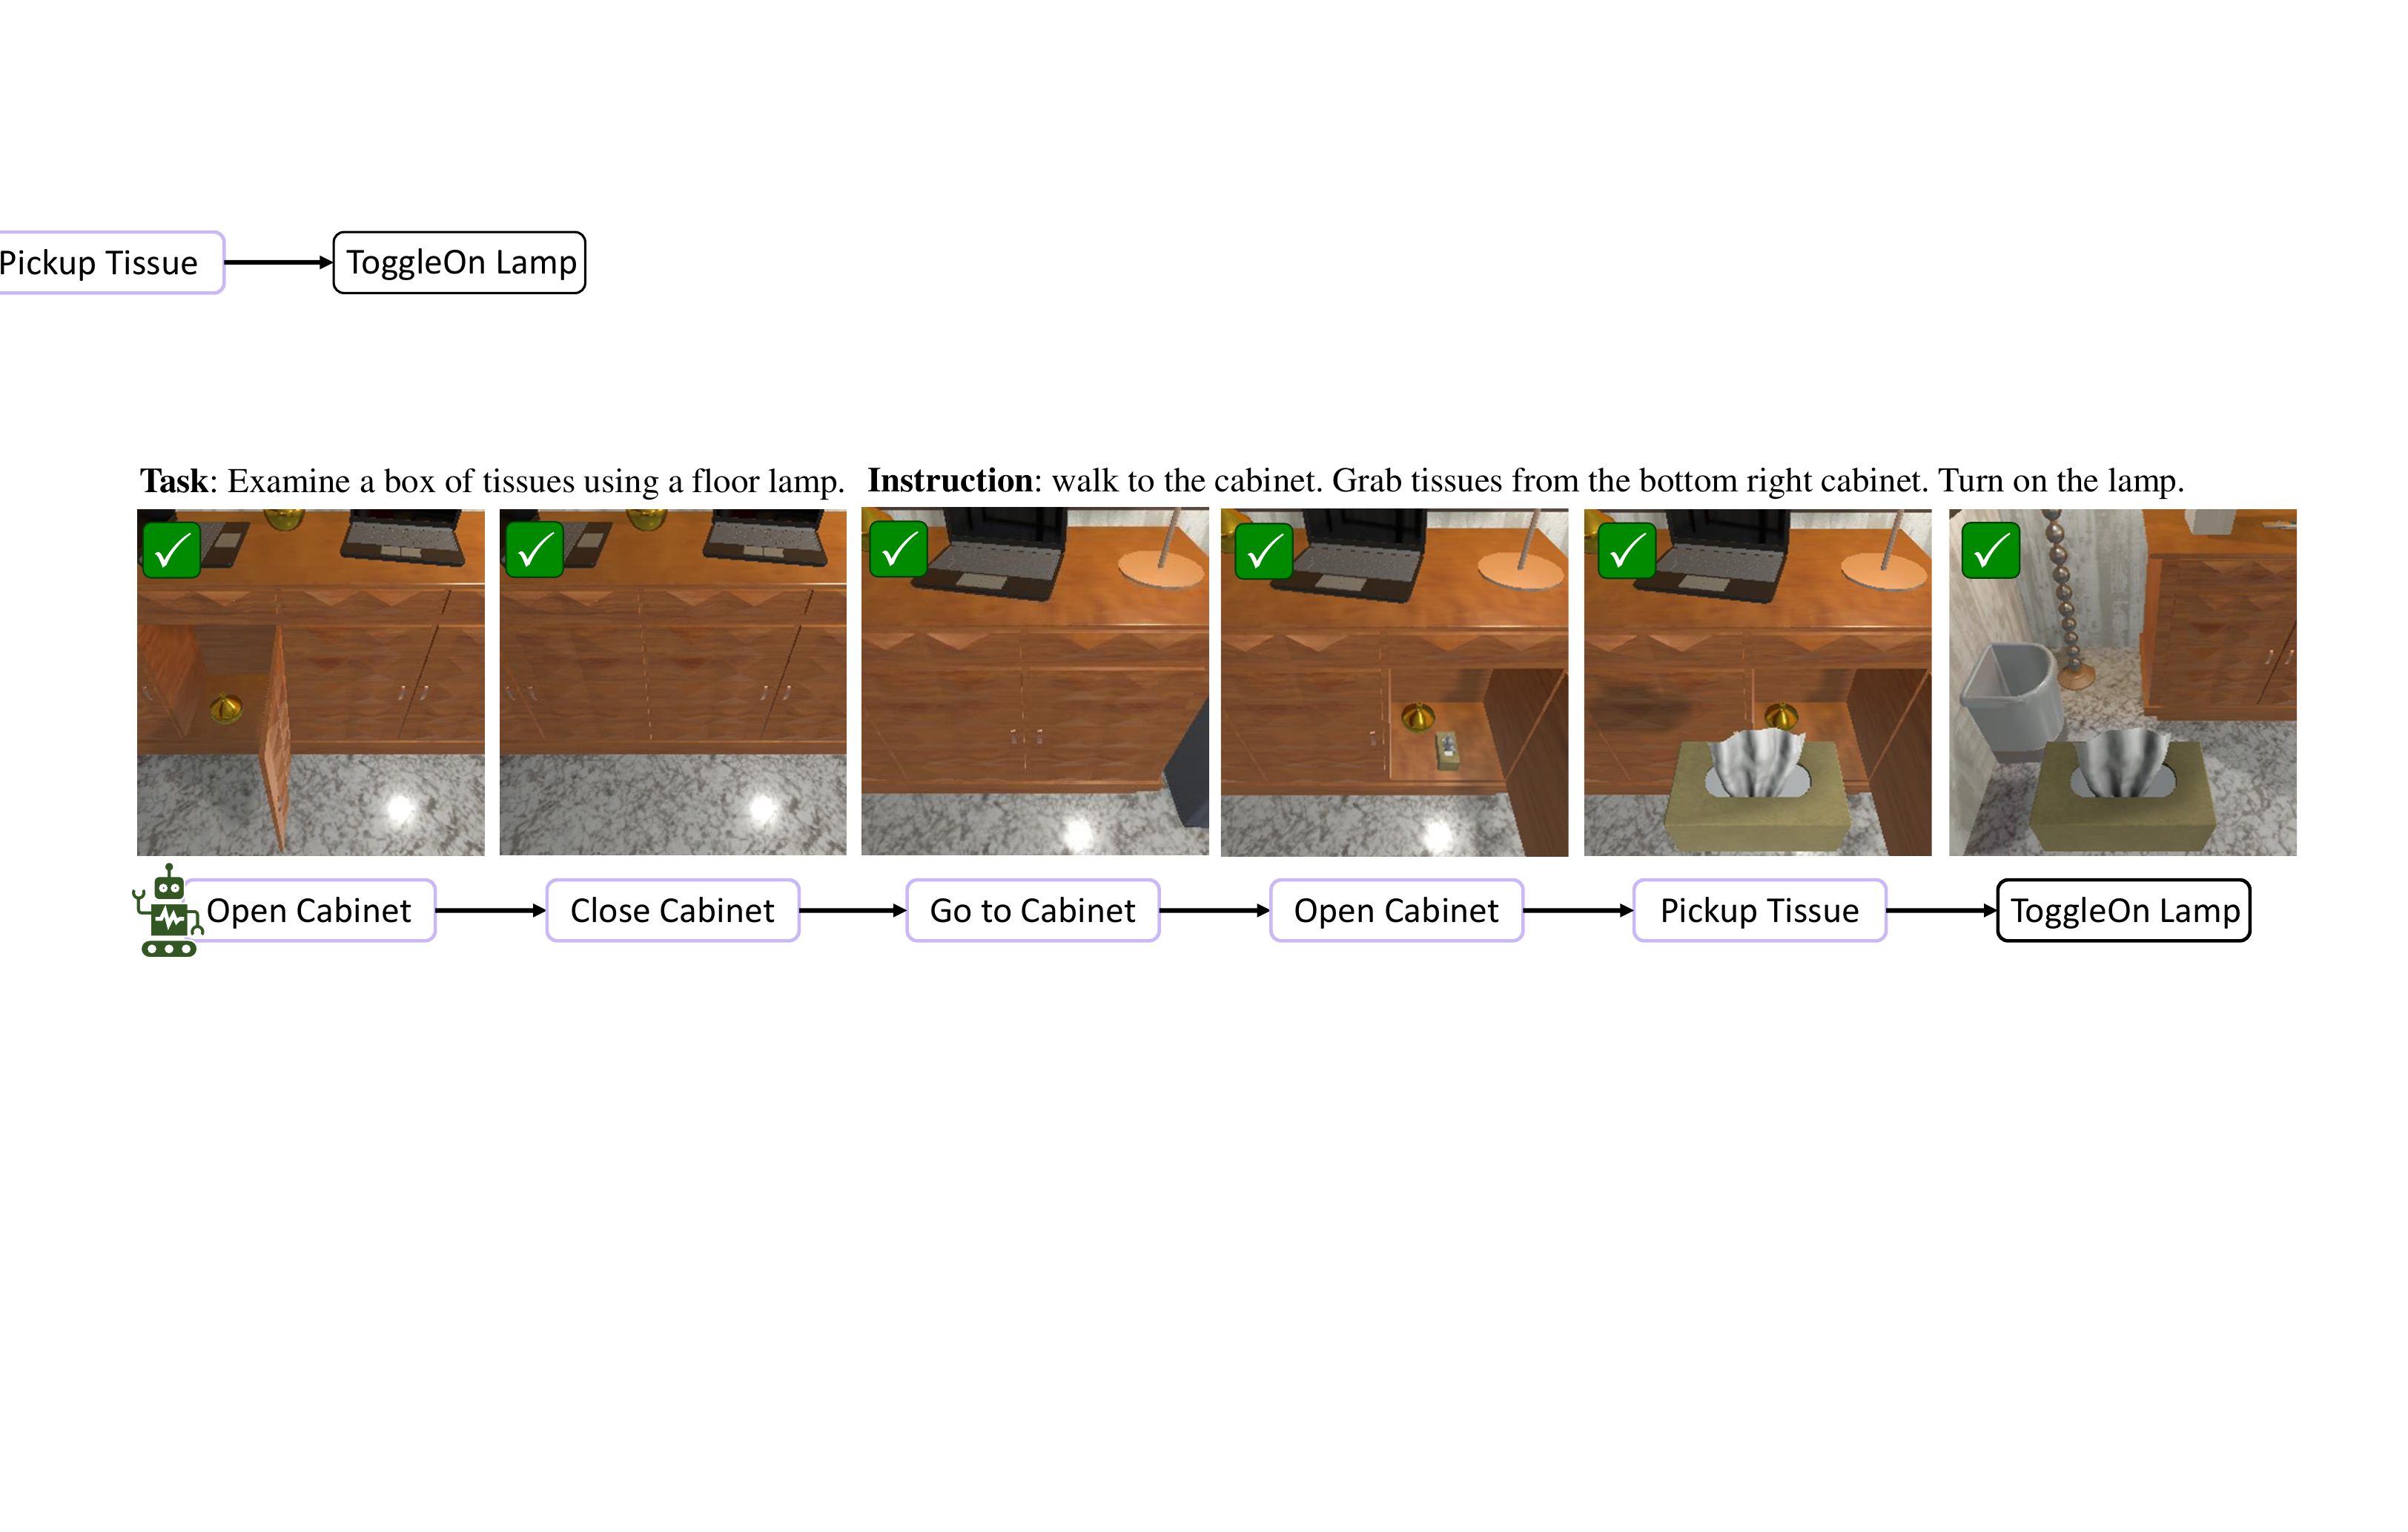}
    \vspace{-0.2cm}
    \caption{Additional visualization of the complete agent action sequence acquired by our ThinkBot, where our method can not only recover the missing actions with interacted instances but also revise the recovered actions when opening the wrong cabinet.}
    % \vspace{-1em}
    \vspace{-0.1cm}
    \label{a:fig:qualitative_a_sequence_2}
\end{figure*}

\begin{figure*}[t!]
    \small
    \centering
    \includegraphics[width=\linewidth]{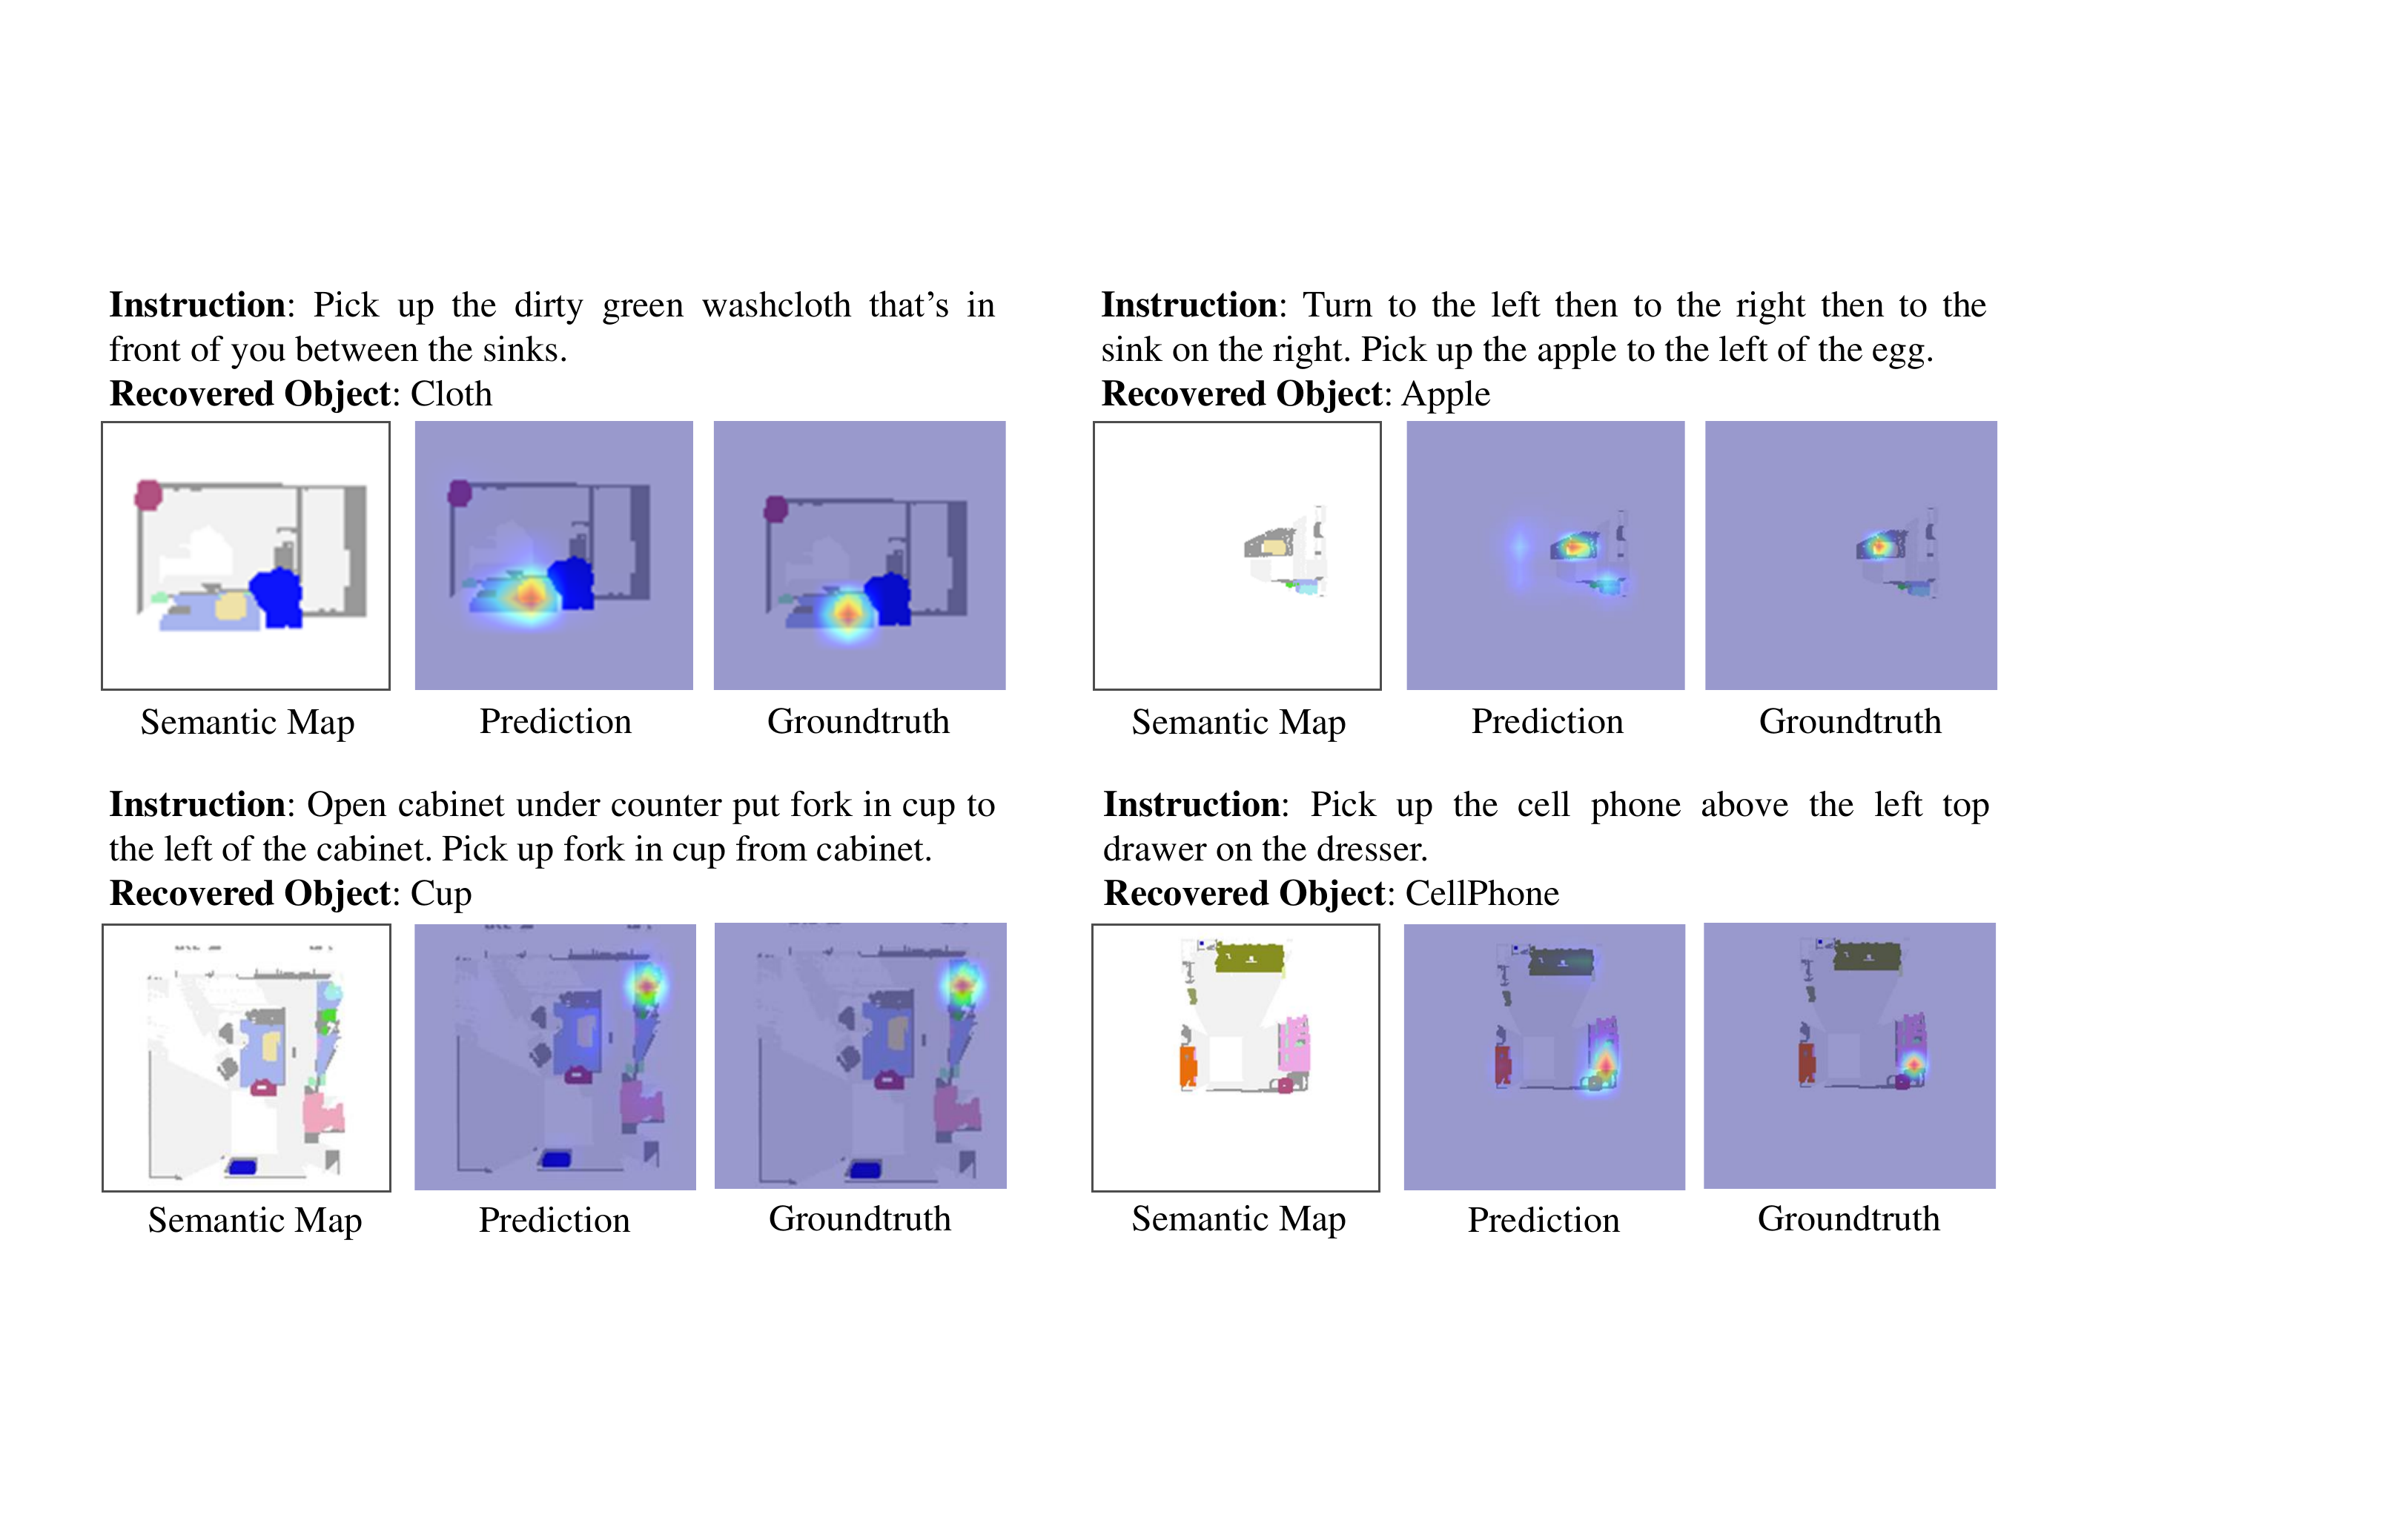}
    \vspace{-0.2cm}
    \caption{Additional visualization of the predicted and groundtruth positions of interacted objects, where the partially observed semantic maps are also depicted.}
    % \vspace{-1em}
    % \vspace{-0.0cm}
    \label{a:fig:qualitative_localizer_1}
\end{figure*}

% \vspace{0.4cm}
\section{Additional Quantitative Analysis}
\label{a:additional_quantitative}

\subsection{Error Mode}

\Cref{a:table:error_modes} presents the absolute ratio of failure cases caused by different factors in FILM, Prompter, and the proposed \method. 
The counterparts' results are taken from their papers \cite{min2022film, inoue2022prompter}.
We categorize failure cases into three types: `Goal object not found', `Interaction failures', and `Navigation failures'. 
In a typical trial, these errors occur in a specific order: `Goal object not found', `Interaction failures', and `Navigation failures'.
To illustrate, when the agent encounters a `Goal object not found' error, it will wander around the environment until \num{10} random errors are generated. 
Hence, we only count the predominant error mode (\ie the error mode at the forefront of the order) if an episode fails due to various reasons.
As depicted in \Cref{a:table:error_modes}, the occurrence of the `goal object not found' error substantially decreases (18.08\% vs. 21.10\%) in our \method by incorporating the recovered coherent human instruction. 
Note that our method does not noticeably impact error modes like `Interaction failures' and `Navigation failures', since these are unrelated to the instruction-following strategy that this paper focuses on.
% The results verify the effectiveness of our method in recovering the missing actions and interacted objects from sparse instructions to prevent the agent from failure, while maintaining a comparable performance in interaction and navigation to the state-of-the-arts.
The results verify the effectiveness of our method in recovering the missing actions to prevent the agent from failure, while maintaining a comparable performance in interaction and navigation to the state-of-the-arts.
% Meanwhile, the `Interaction failures' error is also reduced slightly because the agent can follow the coherent instruction to interact with the target object in the appropriate pose.

\subsection{Performance by Task Type}

We compare the proposed ThinkBot with the state-of-the-art methods on the ALFRED benchmark by task types.
The counterparts include end-to-end method Seq2seq \cite{shridhar2020alfred}, MOCA \cite{singh2021factorizing} and modular methods (HLSM \cite{blukis2022persistent}, FILM \cite{min2022film}, Prompter+).
The compared results are taken from their original papers \cite{shridhar2020alfred, singh2021factorizing, blukis2022persistent, min2022film}.
From \Cref{a:table:task_type}, we can observe that our \method outperforms on almost all task types. For instance, \method surpasses the state-of-the-art method Prompter+ on five out of seven task types by sizable margins. 
Especially, \method succeeds in 40.4\% of `Stack \& Place' tasks, which is an absolute improvement of 8.3\% compared to the state-of-the-art method Prompter+.
While Prompter+ suffers from the sparse human instruction that usually causes execution failure, our \method reasons the thought chain in the sparse human instruction to recover the missing action descriptions, and successfully complete different tasks. 

In `Examine' tasks, the agent is instructed to pick up the target object and toggle on a lamp that is initially off. Since our main focus is not on detecting the status of floor lamps, we adopt a trial-and-error approach by toggling all lamps in the current room following \cite{min2022film, inoue2022prompter}. This random selection approach introduces variability in the success rate of these tasks.
In `Pick 2 \& Place' tasks, the agent is directed to take two instances within the same category and relocate them to a specified location. During the repeated subgoal completion, our language model-based instruction completer may be prone to the hallucination issue, which remains a focus for future improvements.

% \newpage
\lstinputlisting[label={a:system_prompt},breaklines=true,caption={Full system prompt for the instruction completer in our \method. The response format is shown in another listing.}]{sec/prompt/chatgpt_imagination_system_template_v4_open.txt}

\lstinputlisting[label={a:response_format},breaklines=true,caption={The response format of the instruction completer.}]{sec/prompt/action_response_format.txt}

\section{Additional Qualitative Analysis}
\label{a:additional_qualitative}

\subsection{Action Sequence Visualization}
% We present qualitative examples of the generated action sequence in \Cref{fig:qualitative_case_study} from Prompter+ and our ThinkBot. 
% In this case, the agent is instructed to \emph{`Take a knife. Cut the lettuce in the fridge'}. The results show that an agent without the instruction completer struggles to complete the task due to the missing `open' action and interacted object `fridge' in the sparse human instruction.
% In contrast, our \method first reasons the thought chain of human instruction (\ie \emph{`open the fridge, slice the lettuce'}), and then recovers the missing `open' action and interacted object `fridge' from the instruction, thus successfully completes the task.
% The case study demonstrates the effectiveness of the instruction completer in recovering the missing actions and interacted objects from sparse human instruction.
We present two more qualitative examples of the generated action sequences from Prompter+ and our \method in \Cref{a:fig:qualitative_a_sequence}. 
In the left case, the agent is instructed to \emph{`Walk to the safe. Take out the key chain from the safe'}. The results show that the previous agent struggles to complete the task due to the missing `Open' action and interacted object `Safe'.
On the contrary, our \method first reasons the thought chain of human instruction, and then recovers the missing `Open' action and interacted object `Safe' from the instruction, thus successfully completing the task.
In the right case, our \method not only recovers the missing `Open' action and interacted object `Cabinet', but also interacts with the right cabinet instance that contains the green cloth.
The case studies demonstrate the effectiveness of \method in recovering the missing actions and interacted objects from sparse human instruction.

In \Cref{a:fig:qualitative_a_sequence_2}, we also showcase an additional complete action sequence of our \method on the ALFRED valid unseen split.
The agent receives the instruction to `Walk to the cabinet. Grab tissues from the bottom right cabinet'. Our \method can not only recover the missing `Open' actions but also refine the recovered actions.
For instance, our instruction completer outputs `Close cabinet, go to another cabinet, and open cabinet' when the agent mistakenly opens the wrong cabinet.

\subsection{Visualization of the Object Localizer}
In this subsection, we illustrate more groundtruth and the predicted locations of the interacted objects from the object localizer.
\Cref{a:fig:qualitative_localizer_1} shows that the predicted object locations are close to the groundtruth in all cases, which indicates that the object localizer can accurately predict the interacted objects' locations.
In the left two cases, the object localizer can use the spatial information (\eg `in front of you') and the semantic information (\eg `from cabinet') in human instruction to predict the positions of target objects precisely.
In the right two cases of severe partially-observed scenarios (\ie only looking around actions from the spawn position are taken), our object localizer can still predict the heatmap of the small target object accurately.  
% In xx, our localizer is also able to pinpoint a large receptacle.

\subsection{A Video for Complete Trial Visualization}
We provide an additional comprehensive trial visualization in the attached video file (\emph{demo.avi}) selected from the valid unseen split. In the video, the agent is instructed to `Put a mug with a spoon inside of it on the counter.' However, the mug is stored in the fridge. Our \method can recover the missing `Go to Fridge' and `Open Fridge' subgoal and locate the interacted objects precisely, thus completing the task effectively and efficiently.

% top-down, semantic map, w/o graph, w/ graph, groundtruth

% {
%     \small
%     \bibliographystyle{ieeenat_fullname}
%     \bibliography{reference, cpem}
% }
